# Supplementary material for: Bayesian Analysis of fMRI data with Spatially-Varying Autoregressive Orders
Source: arXiv:1710.01434 source file (2017-10-04)
Supplement: Supplementary file 1 [file essay--appendix.tex]

	%This is a sample appendix
\newpage

\subsection*{Appendix}
\label{appx1}

\subsection{Log-likelihood}

Let $c$ denote the normalizing constant, the log-likelihood $l$ can be expressed as:
\begin{eqnarray*}
l&=&\sum_n \sum_t -\frac{\lambda_n}{2} (e_{tn} - \sum_p \tilde e_{ntp} a_{pn})^2 + \frac{T-P}{2} \sum_n \log \lambda_n+c \nonumber \\
&=& \sum_n \sum_t -\frac{\lambda_n}{2} \Big [ (y_{tn}-\sum_k \mb x_{tk}w_{kn})-\sum_p (y_{t-p,n} - \sum_k x_{t-p,k} w_{kn}) a_{pn}  \Big ]^2 \\
&+& \frac{T-P}{2} \sum_n \log \lambda_n +c \\
&=& \sum_n \sum_t -\frac{\lambda_n}{2}  \Big [ \sum_p ( y_{t-p,n} - \sum_k x_{t-p,k} w_{kn}) a_{pn}^*   \Big ]^2 + \frac{T-P}{2} \sum_n \log \lambda_n +c
\end{eqnarray*}

where $a_{pn}^*=a_{pn}$ if $p \neq 0$ and $a_{pn}^*=-1$ otherwise.

\subsection{Priors}
All priors are explicitly given in Chapter \cite{teng2016comparison}, here we add a supplement for $\mathbf a_n$. In practice, when we update $\mathbf a_n$, the spike-and-slab prior are parametrized as follows:
\[
a_{pn} \mid \gamma_{pn} = \gamma_{pn} \mbox N(0, \tau_p^{-1}) + (1-\gamma_{pn}) \mbox N(0,(\epsilon \tau_p)^{-1}) 
\]
where $\epsilon$ is a very large constant so that the spike part has a extremely low variance that approximates point mass at zero. This parametrization can help with the mixing than a pure spike which is an exact point mass at $0$. The log-prior is therefore:
\[
 \log \pi (a_{pn} \mid \gamma_{pn}) =-\frac{\tau_p}{2} a_{pn}^{2} \delta(\gamma_{pn}) + \frac12 \log \tau_p  +\frac{1}{2} \log \delta (\gamma_{pn}) +c 
\]

where $\delta (\gamma_{pn})=\epsilon$ if $\gamma_{pn}=0$ and $1$ otherwise.

\subsection{Posterior distribution}
We derive the posterior distribution for $\mb w_{n}$, $\mb a_{n}$, $\gamma_{pn}$, $\alpha_k$, $\tau_p$, $\lambda_n$. 
\subsubsection{For $\mb w_{n}$}
Let $\mb{\tilde y}_{tn} \equiv (y_{t,n},y_{t-1,n},...,y_{t-P,n})$, $\mb{\tilde x}_{tk} \equiv (x_{t,k},x_{t-1,k},...,x_{t-P,k})$. Then putting $x_k$  together, define $\mb{\tilde X}_t \equiv (\mb{\tilde x}_1^T,...,\mb{\tilde x}_K^T)^T$. We have

\begin{eqnarray*}
\log (\mb w_n | \cdot) &=& \frac{\lambda_n}{2} \sum_t \Big[ (\mb{\tilde y}_{tn} - \mb{\tilde X}_t \mb w_n)^T \mb a_n^*   \Big]^2 -\sum_k \frac{\alpha_k}{2} \mb w_k^T (\mb S^T \mb S) \mb w_k+c \\
&=&-\frac{\lambda_n}{2} \sum_t \Big[  \mb{\tilde y}_{tn} \mb a_n^* - (\mb{\tilde X}_t \mb a_n^*)^T \mb w_n  \Big]^2 - \sum_k \frac{\alpha_k}{2} \mb w_k^T (\mb S^T \mb S)\mb w_k +c\\
&=&-\frac{1}{2} \mb w_n^T \Big[ \lambda_n \sum_t (\mb{\tilde X}_t \mb a_n^*) (\mb{\tilde X}_t \mb a_n^*)^T +(\mb S^T \mb S)_{nn}\mbox{Diag}(\bs \alpha)  \Big] \mb w_n \\
&+& \Big[ \lambda_n \sum_t (\mb{\tilde y}_{tn} \mb a_n^*)(\mb{\tilde X}_t \mb a_n^*) -\bs \alpha   \circ \sum_{n^{\prime} \neq n} (\mb S^T \mb S)_{nn^{\prime}} \mb w_{n^{\prime}} \Big]^T \mb w_n+c
\end{eqnarray*}

where $\mbox{Diag}(\mb v)$ denotes the diagnoal matrix with diagonal elements formed by vector $\mb v$, and $\circ$ denotes Hadamard product.

Thus
\[
\mb w_n \sim \mbox N(\bs \mu_{\mb W}^n, \bs \Sigma_{\mb W}^n )
\]
with
\begin{eqnarray*}
&&\bs \Sigma_{\mb W}^n = \Big[ \lambda_n \sum_t (\mb{\tilde X}_t \mb a_n^*) (\mb{\tilde X}_t \mb a_n^*)^T + (\mb S^T \mb S)_{nn^{\prime}} \mbox{Diag} (\bs \alpha)         \Big]^{-1} \\
&&\bs \mu_{\mb W}^n = \Big [  \lambda_n \sum_t (\mb{\tilde y}_{tn} \mb a_n^*)(\mb{\tilde X}_t^T \mb a_n^*)-\bs \alpha \circ \sum_{n^{\prime} \neq n} (\mb S^T \mb S)_{nn^{\prime}} \mb w_{n^{\prime}}     \Big ] \mb \Sigma_{\mb W}
\end{eqnarray*}

 \subsubsection{For $\mb a_{n}$}
 Denote $\mb{\tilde y}_{tn}^* \equiv (y_{t-1,n},...,y_{t-P,n})$, $\mb{\tilde x}_{tk}^* \equiv (x_{t-1,k},...,x_{t-P,k})$, $\mb{\tilde X}_t^* \equiv (\mb{\tilde x}_1^{*T},...,\mb{\tilde x}_K^{*T})^T$. 
 \begin{eqnarray*}
 \log p(\mb a_n | \cdot)&=&-\frac{\lambda_n}{2} \sum_t \Big[  -(\mb{\tilde y}_{tn}^*-\mb{\tilde X}_t^* \mb w_n)^T \mb a_n +(\mb y_{tn} -\mb X_t \mb w_n)   \Big]^2 -\sum_p \frac{\tau_p}{2} \delta(\gamma_{pn}) a_{pn}^2 \\
 &=&-\frac{1}{2} \mb a_n^T \Big[ \lambda_n \sum_t (\mb{\tilde y}_{tn}^* -\mb{\tilde X}_{tn}^* \mb w_n)(\mb{\tilde y}_{tn}^* - \mb{\tilde X}_t^* \mb w_n)^T +\mbox{Diag} (\bs \tau \circ \delta(\bs \gamma_{n}))    \Big] \mb a_n \\
 &+& \lambda_n ( y_{tn}-\mb X_t \mb w_n) (\mb{\tilde y}_{tn}^* -\mb{\tilde X}_t^* \mb w_n)^T \mb a_n
 \end{eqnarray*}
 
 Thus 
 \[
 \mb a_n \sim \mbox N(\bs \mu_{\mb A}^n, \bs \Sigma_{\mb A}^n)
 \]
 
 with
 \begin{eqnarray*}
 &&\bs \Sigma_{\mb A}^n = \Big[ \sum_t(\mb{\tilde y}_{tn}^* - \mb{\tilde X}_t^* \mb w_n)(\mb{\tilde y}_{tn}^*-\mb{\tilde X}_t^* \mb w_n)^T+\mbox{Diag}(\bs \tau \circ \delta(\bs \gamma_{n}))   \Big]^{-1} \\
 &&\bs \mu_{\mb A}^n = \Big [  \lambda_n \sum_t (y_{tn} - \mb X_t \mb w_n) (\mb{\tilde y}_{tn}^*-\mb{\tilde X}_t^* \mb w_n)^T   \Big] \mb \Sigma_{\mb A}^n
 \end{eqnarray*}

\subsubsection{For $\gamma_{n}$}
\begin{eqnarray*}
p(\gamma_{pn}=1 \mid \cdot )&=&\frac{L(\gamma_{pn}=1) p(\gamma_{pn}=1 \mid \gamma_{-pn})}{L(\gamma_{pn}=1) p(\gamma_{pn}=1 \mid \gamma_{-pn})+L(\gamma_{pn}=0) p(\gamma_{pn}=0 \mid \gamma_{-pn})}  \\
&=& \frac{L(\gamma_{pn}=1)/L(\gamma_{pn}=0) \exp \Big \{ \beta_{0p}+\beta_{1p} \sum_{n^{\prime} \sim n} \gamma_{pn^{\prime}} \Big\} }{L(\gamma_{pn}=1)/L(\gamma_{pn}=0) \exp \Big \{ \beta_{0p}+\beta_{1p} \sum_{n^{\prime} \sim n} \gamma_{pn^{\prime}} \Big\} +1}
 \end{eqnarray*}
 
 where $L(\gamma_{pn})$ is the likelihood associated with $\gamma_{pn}$. So we have:
 \begin{eqnarray*}
 \frac{L(\gamma_{pn}=1)}{ L(\gamma_{pn}=0) }= \exp \Big \{-\frac{\tau_p}{2} a_{pn}^2 + \frac{\epsilon \tau_p}{2} a_{pn}^2 - \frac{1}{2} \log \epsilon     \Big \} \\
 =\exp \Big \{ \frac{(\epsilon-1)\tau_p}{2} a_{pn}^2 -\frac{1}{2} \log \epsilon   \Big \}
 \end{eqnarray*}

 Thus
 \[
 \gamma_{pn}  \sim \mbox{Ber}(p(\gamma_{pn}=1 \mid \cdot))
 \]

 \subsubsection{Swendsen-Wang update of $\gamma_p$}
 \begin{enumerate}
 \item For any pair of neighbors $(n_1,n_2)$ that $\gamma_{pn_1}=\gamma_{pn_2}$, form bonds with probability $1-\exp(-\beta_{1p})$. \\
 \item Let $\{n\}$ denote the set of voxels that belong to one common cluster. For each of the cluster $\{n\}$, calculate:
 \begin{eqnarray*}
 p(\gamma_{p\{n\}}&=&1 \mid \cdot)=\frac{L(\gamma_{p\{n\}}=1) \exp \Big \{ \beta_0 \sum_{n \in \{n\}} \gamma_{pn}\Big\}}{L(\gamma_{p\{n\}}=1) \exp \Big \{ \beta_0 \sum_{n\in \{n\}} \gamma_{pn}\Big\}+L(\gamma_{p\{n\}}=0)} \\
 &=&  \frac{L(\gamma_{p\{n\}}=1)/L(\gamma_{p\{n\}}=0) \exp \left\{ \beta_0 \sum_{n \in \{n\}} \gamma_{pn}   \right\}}{L(\gamma_{p\{n\}}=1)/L(\gamma_{p\{n\}}=0) \exp \left\{ \beta_0 \sum_{n \in \{n\}} \gamma_{pn}   \right\}+1} \\
 &=& \frac{ \exp \left\{ \beta_0 \sum_{n \in \{n\}} \gamma_{pn} + \frac{1}{2} (\epsilon-1)\tau_p \sum_{\{n\}} a_{p\{n\}}^2 -\sum_{\{n\}} \frac{1}{2} \log \epsilon     \right\} }{\exp \left\{ \beta_0 \sum_{n \in \{n\}} \gamma_{pn} + \frac{1}{2} (\epsilon-1)\tau_p \sum_{\{n\}} a_{p\{n\}}^2 -\sum_{\{n\}} \frac{1}{2} \log \epsilon     \right\}+1}
 \end{eqnarray*}
 where $L(\gamma_{p\{n\}}=1)$ and $L(\gamma_{p\{n\}}=0)$ is the likelihood associated with $\gamma_{p\{n\}}$.
\end{enumerate}

 \subsubsection{For $\alpha_k$}

 \[
 \alpha_k  \sim G\Big(\frac{N}{2} +q_1-1, \Big[\frac12 \mb w_k^T (\mb S^T \mb S) \mb w_k +\frac{1}{q_2} \Big]^{-1}\Big)
 \]
 
 \subsubsection{For $\tau_p$}
 \begin{eqnarray*}
\log p(\tau_p | \cdot) &=& \sum_n \left[ -\frac{\tau_p}{2} a_{pn}^2 \delta(\gamma_{pn}) +\frac{1}{2} \log \tau_p  \right] +(u_1-1) \log \tau_p - \tau_p /u_2 \\
&=& \left(\frac{N}{2} +u_1-1   \right) \log \tau_p - \left(  \frac{1}{2} \sum_n a_{pn}^2 \delta(\gamma_{pn}) +\frac{1}{u_2}  \right ) \tau_p
 \end{eqnarray*}

 \[
 \tau_p \sim  \mbox G\left(\frac{N}{2} +u_1-1, \frac{1}{2}\sum_n a_{pn}^2 \delta(\gamma_{pn}) +\frac{1}{u_2}  \right)
 \]
 
\subsubsection{For $\lambda_n$}

 \[
 \lambda_n   \sim \mbox G\Big(\frac{T-P}{2}+r_1-1,\Big(\frac12\sum_t\Big[\sum_p\Big(y_{t-p,n}-\sum_k x_{t-p,k}w_{kn}\Big)a_{pn}^*\Big]^2+\frac{1}{r_2}\Big)^{-1}\Big)
 \]

 \subsection{Updating Scheme}
The parameter are updated according to the following sequence:
\begin{enumerate}
\item Update $\mb w_{n}$ for $ n=1,...,N$
\item Update $\mb a_{n}$ for $n=1,...,N$.
\item Update $\bs \gamma_{p}$ for $p=1,...,P$ 
\item Update $\alpha_k$ for $k=1,...,K$.
\item Update $\tau_p$ for $p=1,,,.P$.
\item Update $\lambda_n$ for $n=1,...,N$
\item Repeat step 1-6 for sufficiently long time.
\end{enumerate}

\subsection{Proof of neighboring pairs}
Since the length of the cubic is $V_p$, and the neighbors are all $1^{st}$ order neighbors. It is easy to show that:\\
The number of voxels having $3$ neighbors is 8 \\
The number of voxels having $4$ neighbors is $12(V_p-2)$ \\
The number of voxels having $5$ neighbors is $6(V_p-2)^2$. \\
The number of voxels having $6$ neighbors is $(V_p-2)^3$

Thus, the total number of neighbors are
\[
\frac{1}{2}[6(V_p-2)^3+30(V_p-2)^2+48(V_p-2)+24]
\]

which is exactly $3V_p^2(V_p-1)$.
